# Supplementary material for: Local Discovery by Partitioning: Polynomial-Time Causal Discovery Around Exposure-Outcome Pairs
Source: arXiv:2310.17816 source file (2024-06-01)
Supplement: Supplementary file 1 [file appendix_causal_sufficiency.tex]

\subsection{Weakening the causal sufficiency assumption}
\label{sec:appendix_latent}

Here, we show that 1) for arbitrary $\z$, Condition \ref{cond:sufficient_4} can be weakened by introducing Assumptions \ref{assumption:z5_or_no_latents}–\ref{assumption:no_latents_z}; and 2) when $\z$ is pretreatment, LDP is robust to causal insufficiency in $\g$ with only Assumption \ref{assumption:z5_or_no_latents}. 

\subsubsection{Discovery of $\z_5$ indicates valid adjustment under latent confounding of $X$ and $Y$}

Given arbitrary $\z$ with pre- and post-treatment variables, we prove that the theoretical guarantees of LDP hold when Condition \ref{cond:sufficient_4} is replaced with the following three assumptions.

%Proposition \ref{prop:z5_indicates_latents} states the following: \textit{Under Assumptions \ref{assumption:z5_or_no_latents}–\ref{assumption:no_latents_z}, if LDP discovers at least one $Z_5$, then the inferred $\z_1$ is a valid adjustment set, as $\z_5$ is not d-separable from $Y$ unless all backdoor paths are blocked (Algorithm \ref{alg:method}, Step 5). If no $Z_5$ are discovered, the inferred $\z_1$ is still guaranteed to be a valid adjustment set if there are no unobserved members of $\z_1$ except those that lie on backdoor paths that are blocked by conditioning on all discoverable members of $\z_1$.}

\begin{proof}
    If there are unblocked backdoor paths from $X$ to $Y$, $\z_5$ will not be identifiable by LDP. If we assume the existence of a $Z_5 \in \z$, failure to discover this $Z_5$ can be used as an indicator for the presence of unblocked backdoor paths and the valid adjustment set is deemed \textit{unidentifiable}. By extension, if at least one $Z_5$ is discovered, then the resulting $\z_1$ is a valid adjustment set, as all backdoor paths are blocked. If we do not assume the existence of a $Z_5$, then $\z_1$ is only guaranteed to be a valid adjustment set if we assume that all backdoor paths can be blocked by the discoverable members of $\z_1$. 

    As these assumptions do not imply the existence of inter-partition active paths and therefore do not violate Condition \ref{cond:sufficient_1}, all theoretical guarantees hold for partition correctness and valid adjustment set discovery.
\end{proof}

Empirically, we also show that some violations of Assumptions \ref{assumption:no_latents_xy} and \ref{assumption:no_latents_z} do not interfere with our theoretical guarantees (Section \ref{sec:empirical_results}). We leave full characterization of the allowable forms of causal insufficiency in arbitrary $\z$ to future work. 

\subsubsection{LDP is correct under causal insufficiency in $\g$ when $\z$ is pretreatment and contains no M-structures}

Finally, we prove that by taking the standard pretreatment assumption such that $\z \coloneqq \z_1 \cup \z_4 \cup \z_5$ (Figure \ref{fig:pretreatment_only}),  our original theoretical guarantees hold by replacing Condition \ref{cond:sufficient_4} with Proposition \ref{prop:z5_indicates_latents} under \textit{only} Assumption \ref{assumption:z5_or_no_latents} and no other assumptions on causal insufficiency. In this setting, Condition \ref{cond:sufficient_2} is also unnecessary. Numerical validation of these theoretical results is provided in Section \ref{sec:latent}, along with illustrative figures.

\input{figure_tex/figure_pretreatment_only}

Theorem \ref{theorem:pretreatment_latents} states the following:
\textit{Given Proposition \ref{prop:z5_indicates_latents} under only Assumption \ref{assumption:z5_or_no_latents} and no other assumptions on causal sufficiency in $\g$, all theoretical guarantees of LDP hold.}

Proof of Theorem \ref{theorem:pretreatment_latents} follows from Proposition \ref{prop:z5_indicates_latents}, Lemma \ref{lemma:z4_latents}, and Lemma \ref{lemma:z5_latents}. As these lemmas do not imply the existence of inter-partition active paths and therefore do not violate Condition \ref{cond:sufficient_1}, all theoretical guarantees hold for both partition correctness and valid adjustment set discovery.

\begin{lemma}[When $\z$ is pretreatment, discovery of $\z_4$ is not impacted by causal insufficiency in $\g$] \label{lemma:z4_latents}
\end{lemma}

\begin{proof}
    The test for $\z_4$ relies only on knowledge of $X$ and $Y$ ($X \ind Z$ and $X \nind Z | Y \iff Z \in \z_4$). No latent confounding in $\z$ could render any true $Z_4$ marginally dependent on $X$ without violating the definition of $\z_4$ (Definition \ref{def:z4}). This implies that a member of $\z_4$ cannot share a latent confounder with nor be confounded by a member of $\z_1$ nor $\z_5$. Thus, we only need to consider the case where latent confounding in $\z_4$ involves other members of $\z_4$. Per Proposition \ref{prop:path_1}, $X \nind Z_4 | Y$ remains true even if additional active paths are added to $\g$, as the conditioning set ($Y$) remains unchanged. Thus, unobserved confounded paths within $\z_4$ cannot impact the discovery of the observed $\z_4$.
\end{proof}

\begin{lemma}[When $\z$ is pretreatment, discovery of $\z_5$ is not impacted by causal insufficiency in $\g$] \label{lemma:z5_latents}
\end{lemma}

\begin{proof}
    We will show that the three possible cases of latent confounding for $\z_5$ have no impact on its discovery: 1) a $Z_5$ and $Y$ are latently confounded, 2) a $Z_5$ and $X$ are latently confounded, and 3) a $Z_5$ and another member of $\z$ are latently confounded. 

    \textit{Case 1.} This setting is impossible, as no true $Z_5$ can share a latent confounder with $Y$ by definition; if so, the putative $Z_5$ would actually be in $\z_1$ (Definition \ref{def:z5}). In this scenario, the putative (false) $Z_5$ can never be placed in $\z_5$ at Step 7, as it will always be marginally dependent on at least one other $Z_1$ (e.g., its confounder with $Y$).
    
    \textit{Case 2.} Only two partitions allow for an edge into $X$: $\z_1$ and $\z_5$. However, no member of $\z_1$ can act as a confounder for a $Z_5$ and any other variable, as this would violate the definition of $\z_5$ by introducing an active path from $\z_5$ to $Y$ that is not mediated by $X$ (Definition \ref{def:z5}). Therefore, only another $Z_5$ can act as a confounder for $\z_5$ and $X$. Latent confounding by another $Z_5$ would render the $Z_5$ in question a proxy or surrogate instrument, a known variant of the instrumental variable \citep{hernan_instruments_2006, lousdal_introduction_2018}. Failure to observe such a latent $Z_5$ would have no effect on Steps 5–7 of Algorithm \ref{alg:method}, as the latent variable could not lie on any backdoor paths from $X$ to $Y$ by definition (Figure \ref{fig:z5_z1}). 

    \textit{Case 3.} $\z_5$ can never share latent confounders with $\z_4$, as this would violate the definitions of both $\z_4$ and $\z_5$ (Definitions \ref{def:z4}, \ref{def:z5}). As proven under Case 2, a member of $\z_5$ and a second variable cannot be latently confounded by a member of $\z_1$ without violating the definition of $\z_5$. Thus, we only need to consider the substructure $Z_5 \leftarrow \cdots U \cdots \rightarrow Z$ where $U \in \z_5$ and $Z \in \z_5 \cup \z_1$. This setting is analogous to the proxy instrument described under case 2, where the unmeasured instrument does not lie on a backdoor path between $X$ and $Y$ and therefore cannot interfere with Steps 5–7 of Algorithm \ref{alg:method}. 
\end{proof}

\subsection{Empirical robustness to latent confounding} 
\label{sec:latent} 

\input{figure_tex/figure_latent}

\begin{table}[!h]
    \centering
    \begin{adjustbox}{max width=\textwidth}
    \begin{tabular}{l c c c c c c}
    \toprule
    & \multicolumn{3}{c}{\textsc{Figure \ref{fig:latent_experiments} (left)}} & \multicolumn{3}{c}{\textsc{Figure \ref{fig:latent_experiments} (right)}} \\
    %\cmidrule(lr){2–4}  \cmidrule(lr){5–7} 
    %%%%
    \textsc{Latent Confounder} & None & $Z_{5a}$ & $Z_{4a}$ & None & $Z_{5b}$ & $Z_{4b}$ \\
    \midrule
    \textsc{Label Accuracy} & 98.2 (97.7–98.7) & 100 (100–100) & 100 (100–100) & 100 (100–100) & 100 (100–100) & 100 (100–100) \\
    \bottomrule
    \end{tabular}
    \end{adjustbox}
    \caption{Performance of LDP for causally insufficient linear–Gaussian DAGs (Figure \ref{fig:latent_experiments}) with pretreatment $\z$ numerically validates Theorem \ref{theorem:pretreatment_latents}. Label accuracy is computed with the expected label for LDP under causal sufficiency as the ground truth. This is to accommodate the fact that LDP is \textit{expected} to mislabel $Z_{1a}$ and $Z_{1c}$ as $\z_{\textsc{Post}}$ even when there are no latent variables in $\g$, though the returned $\z_1$ ($\{Z_{1b}\}$) is still expected to be a valid adjustment set. All other variables in Figure \ref{fig:latent_experiments} are expected to have correct partition labels. Accuracies are averaged over 100 replicate DAGs with identical structure and varying coefficients, with structural equations reported in Table \ref{tab:sem_continuous}. The 95\% confidence intervals are reported in parentheses. Independence is determined by Fisher-z tests ($\alpha = 0.005$). All experiments were run on a 2017 MacBook with 2.9 GHz Quad-Core Intel Core i7.}
    \label{tab:latent_pretreatment}
\end{table}

\paragraph{M-structures and Butterfly Structures} We probed the robustness of LDP to specific forms of latent confounding in $\g$ that contain M-structures or butterfly structures \citep{ding_adjust_2014} and post-treatment variables. Each experiment tested 100 replicate 13-node, linear-Bernoulli DAGs (Figure \ref{fig:m_butterfly}) using chi-square tests ($\alpha = 0.001$). In DAGs with M-structures where node $M_1 \in \z_5$ is latent, partition accuracy was 99.8\% (95\% CI $[99.4,100]$), $\z_1$ precision and recall were 99.0\%  (95\% CI $[97.0,100]$), and M-colliders were correctly labeled. With $M_2 \in \z_4$ latent, partition accuracy was 80.0\% (95\% CI $[80.0,80.0]$), $\z_1$ precision was 33.3\% (95\% CI $[33.3,33.3]$), and $\z_1$ recall was 100.0\%, as the M-collider was placed in $\z_1$. In such a case, $\mathbf{A}_{XY}$ could induce M-bias \citep{ding_adjust_2014}. Treating butterfly nodes $\{B_1,B_2\} \in \z_1$ as latent had no effect on performance. With $B_3 \in \z_1$ unobserved, partition accuracy was 80.0\% (95\% CI $[80.0,80.0]$) and $\z_1$ precision and recall were 66.7\% (95\% CI $[66.7,66.7]$), leaving an unblocked backdoor path $X - B_3 - Y$. These results indicate that causal sufficiency in $\g$ is not a necessary condition when $\z$ is not pretreatment, but certain forms of latent confounding are detrimental to both partition accuracy and valid adjustment set identification.

\clearpage
