# Supplementary material for: Local Discovery by Partitioning: Polynomial-Time Causal Discovery Around Exposure-Outcome Pairs
Source: arXiv:2310.17816 source file (2024-06-01)
Supplement: Supplementary file 2 [file appendix_valid_no_latents.tex]

\subsection{Validity of adjustment sets under causal sufficiency}

To provide additional intuition for how LDP discovers VAS, we provide further proofs for the setting of causal \textit{sufficiency} and arbitrary inter-partition active paths.

We begin by proving that the identification of $\z_4$ and $\z_5$ is guaranteed in this setting (Theorem \ref{theorem:z4_z5_guaranteed}), as the existence of these partitions is sufficient for discovering $\z_1$ under conditions \ref{cond:sufficient_2} and \ref{cond:sufficient_3}. We prove \ref{item:valid_1} with Lemma \ref{lemma:desc_x} by demonstrating that all $Z$ placed in $\z_1$ are non-descendants of $X$, even if their partition label is incorrect. By extension, proving \ref{item:valid_1} guarantees that no causal path from $X$ to $Y$ will be blocked by the $\z_1$ returned by LDP. We prove \ref{item:valid_2} with Theorem \ref{theorem:blocked_c1_violated}, which states that LDP blocks all backdoor paths even when condition \ref{cond:sufficient_1} is violated.  

\subsubsection{Identification of $\z_4$ and $\z_5$ is guaranteed}

In order to catch $\z_5$, LPD must first catch all $\z_2$ that, when conditioned on, open an active path from $X$ to $Y$. In order to catch such $\z_2$ at Step 4, LDP must first catch $\z_4$ at Step 2. Therefore, we must prove that each of these steps are unaffected by inter-partition active paths. 

\begin{theorem}[Identification of $\z_4$ and $\z_5$ is guaranteed when sufficient condition \ref{cond:sufficient_1} is violated] \label{theorem:z4_z5_guaranteed} 
\end{theorem}

Proof of Theorem \ref{theorem:z4_z5_guaranteed} follows from Lemmas \ref{lemma:z4_inter} and \ref{lemma:z5_inter}.

\begin{lemma}[Discovery of $\z_4$ is guaranteed at Step 2] \label{lemma:z4_inter}
\end{lemma}

\begin{proof}
    The test at Step 2 of Algorithm \ref{alg:method} relies only on $\{X,Y,Z\}$ for a given candidate $Z$. No valid inter-partition active paths can cause $\z_4$ to be marginally dependent on $X$, as this would violate the definition of $\z_4$ (Definition \ref{def:z4}). Per Proposition \ref{prop:path_1}, no valid inter-partition active paths can negate the conditional dependence of $\z_4$ and $X$ as the conditioning set remains unchanged. Therefore, the discovery of $\z_4$ remains unaffected by inter-partition active paths.  
\end{proof} 

\begin{lemma}[Discovery of $\z_5$ is guaranteed at Step 5]  \label{lemma:z5_inter}
%[Discovery of $\z_2$ that are descendants of $X$ or $Y$  is guaranteed at Step 4] This guarantees that any $Z_2$ that opens an inactive path between $X$ and $Y$ when conditioned on (rendering it active) is guaranteed. Thus, such $\z_2$ cannot interfere with the discovery of $\z_5$ at Step 5.
\end{lemma}
\vspace{-3mm}
\begin{proof}
    To prove Lemma \ref{lemma:z5_inter}, we will show that each phase to the discovery of $\z_5$ at Steps 5, 6, and 7 is not affected by violations of sufficient condition \ref{cond:sufficient_1}.
    
    First, we address potential impacts at Step 5. A subset of $\z_2$ is the only subpartition whose inclusion in the conditioning set at Step 5 can prevent downstream detection of $\z_{5}$. %This problematic subset of $\z_2$ is conditionally independent of $Y$ given $X \cup \z'$, where $\z'$ contains members of $\z_1$ and $\z_3$ that are adjacent to $Y$ (among other variables).
    This problematic subset of $\z_2$ must be 
    \begin{enumerate}[noitemsep,topsep=0pt]
        \item marginally independent of all of $\z_4$, otherwise it would be identified at Step 4; and
        \item able to render an inactive path between $X$ and $Y$ active by its inclusion in the conditioning set at Step 5.
    \end{enumerate}
    We will show that no $Z_2$ that is undiscovered by Step 4 can meet the second condition. Observe that any $Z_2$ can either be descended from $Y$ or share only a confounded path with $Y$. To meet the first condition above, a $Z_2$ cannot be descended from $Y$. %$\z_2$ and $\z_6$ are the only partitions that can be descended from $Y$. If a $Z_2$ is descended from $Y$, it can either be 1) directly adjacent to $Y$, 2) descended from another $Z_2$, or 3) descended from a $Z_6$. 
    Any $Z_2$ that is a descendant of $Y$ will always be discovered at Step 4 regardless of the other paths it lies on, as it will always be marginally dependent on $\z_4$. 

    We next consider the subset of $\z_2$ that only shares confounded paths with $Y$. For a $Z_2$ to meet the second condition above, any path between $X$ and $Y$ that is opened by conditioning on this $Z_2$ \textit{must not be re-blocked} by the rest of the conditioning set used in Step 5. Thus, we must prove that any $Z_2$ that is not identified at Step 4 must be on a path to $Y$ that is \textit{re-blocked} by the other members of the conditioning set at Step 5.
    
    Consider the types of confounded paths that $\z_2$ can share with $Y$. Any confounder for $\{Z_2,Y\}$ can only belong to $\z_1$, $\z_3$, $\z_4$, or $\z_6$. This follows from Table \ref{tab:path_grid}, which states that the only partitions that can have an edge entering $Y$ are:
    \begin{enumerate}[noitemsep,topsep=0pt]
        \item Type 2 paths to $Y$: $\z_1$, $\z_3$, $\z_4$.
        \item Type 4 paths to $Y$: $\z_1$, $\z_2$, $\z_4$.
        \item Type 5 paths to $Y$: $\z_1$, $\z_3$, $\z_4$.
        \item Type 6 paths to $Y$: $\z_2$, $\z_6$.
    \end{enumerate}
    If the confounder for $\{Z_2,Y\}$ is in $\z_4$ (e.g., in the M-structure featured in Figure \ref{fig:m_butterfly}), then this $Z_2$ is guaranteed to be discovered at Step 4. Likewise, as $\z_6$ is descended from $\z_4$ through $Y$, any $Z_2$ sharing an active path with $\z_6$ will be discovered at Step 4. If the only confounders for $\{Z_2,Y\}$ are in $\z_1$ or $\z_3$, $Z_2$ will not be discovered at Step 4 and will be conditioned on during Step 5. However, all members of $\z_1$ and $\z_3$ that are adjacent to $Y$ will also be included in the conditioning set at Step 5. Together with $X$, these variables will block all paths from $\z_5$ to $Y$. Therefore, such a $Z_2$ will be on a path to $Y$ that is \textit{re-blocked} by the conditioning set at Step 5. 

    Finally, we address the resolution of $\z_5$ at Steps 6 and 7 when sufficient condition \ref{cond:sufficient_1} does not hold. Even when \ref{cond:sufficient_1} is violated, no $Z_5$ will ever be dependent on a $Z_1$ that is directly adjacent to $Y$ (as described in Definition \ref{def:z5} and Proposition \ref{prop:z5_z1_collider}). Therefore, any $Z_5$ will be placed in $\z_{1,5}$ at Step 6 and in $\z_5$ at Step 7.
\end{proof}

%\subsubsection{LDP does not place descendants of $X$ in $\z_1$}

\subsubsection{Adjustment sets returned by LDP block all backdoor paths for $\{X,Y\}$}

\begin{theorem}
    [Adjustment sets returned by LDP block all backdoor paths for $\{X,Y\}$ when sufficient condition \ref{cond:sufficient_1} is violated] \label{theorem:blocked_c1_violated}
\end{theorem}

Proof of Theorem \ref{theorem:blocked_c1_violated} proceeds from the following argument, as supported by Lemmas \ref{lemma:catch_one_z1_per_path} and \ref{lemma:final}. 

As illustrated in Figure \ref{fig:backdoor}, not every $Z_1$ must be included in the adjustment set in order to block all backdoor paths. We will show that the adjustment set returned by LDP still blocks all backdoor paths even when 1) some ground truth $Z_1$ are not placed in $\z_1$ and 2) some non-$Z_1$ are placed in $\z_1$.

First, we address the latter claim that LDP returns VAS even when some non-$Z_1$ are placed in $\z_1$. Consider the partitions that could be incorrectly labeled as $\z_1$ when sufficient condition \ref{cond:sufficient_1} is violated. We have already proven that no descendant of $X$ will ever be placed in $\z_1$ (Lemma \ref{lemma:desc_x}). This implies that members of $\z_3$, $\z_6$, and $\z_7$ can never be mislabeled as $\z_1$. $\z_8$ can also never be placed in $\z_1$, as inter-partition active paths have no effect on its discovery at Step 1. This leaves $\z_2$, $\z_4$, and $\z_5$. Per Theorem \ref{theorem:z4_z5_guaranteed}, violating sufficient condition \ref{cond:sufficient_1} does not impact discovery of $\z_4$ and $\z_5$. Further, these variables are permissible in VAS and are intentionally retained under some criteria (e.g., the disjunctive cause criterion \citep{vanderweele_new_2011}). Per Lemma \ref{lemma:z5_inter}, $\z_2$ can only share a confounded path with $Y$ when the confounder is in $\z_1$, $\z_3$, $\z_4$, or $\z_6$. Further, any $Z_2$ that is marginally dependent on a $Z_4$ or $Z_6$ will be placed in $\z_{\textsc{Post}}$ at Step 4. Per Lemma \ref{lemma:desc_x}, any member of $\z_2$ that is descended from $X$ will never be placed in $\z_1$. Thus, when a $Z_3$ acts as a confounder for a $Z_2$ and $Y$, this $Z_2$ will never be placed in $\z_1$. Therefore, the only members of $\z_2$ that could be placed in $\z_1$ are non-descendants of $X$ whose only path to $Y$ is confounded by members of $\z_1$.  This does not violate the validity of the returned adjustment set, as such $Z_2$ lie on paths that will already by blocked by the rest of $\z_1$, preventing collider bias. This case is illustrated by node $Z_2^2$ in Figure \ref{fig:z4_z5_z1_paths} (right-hand DAG).

Next, we address the former claim that the adjustment set returned by LDP still blocks all backdoor paths even when some ground truth $Z_1$ are mislabeled.  We begin by introducing the concepts of \textit{root}-$Z_1$ and \textit{collider}-$Z_1$. We observe that every backdoor path features a $Z_1$ that acts as a \textit{root} node for that path: i.e., it is a common cause for $\{X,Y\}$ and all $Z_1$ that are its descendants on the paths to $X$ and $Y$. In Figure \ref{fig:z4_z5_z1_paths}, $\{Z_1^1, Z_1^3, Z_1^6\}$ are roots for backdoor paths in the left-hand DAG while $\{Z_1^2, Z_1^4, Z_1^5\}$ are roots for backdoor paths in the right-hand DAG. When multiple backdoor paths in $\g$ overlap (i.e., share subpaths), some $Z_1$ can behave as \textit{colliders} for two parent $Z_1$. In Figure \ref{fig:z4_z5_z1_paths}, $\{Z_1^2, Z_1^4\}$ are \textit{collider}-$Z_1$ on overlapping backdoor paths in the left-hand DAG while $\{Z_1^1, Z_1^2, Z_1^3\}$ are \textit{collider}-$Z_1$ for backdoor paths in the right-hand DAG. Note that node $Z_1^2$ in the right-hand DAG simultaneously behaves as a \textit{root}-$Z_1$ and a \textit{collider}-$Z_1$ for different backdoor paths.

Let $\mathbf{A}_{XY}$ be an adjustment set for $\{X,Y\}$ that is returned by LDP. We claim that any $\mathbf{A}_{XY}$ that blocks a backdoor path $\mathcal{P}$ meets \textit{at least one} of the following conditions with respect to $\mathcal{P}$: 
\begin{enumerate}[noitemsep,topsep=0pt,label={\itshape Item \arabic*},leftmargin=\widthof{[Item 1]}+\labelsep]
    \item\label{item:z1_collider_1} At least one non-\textit{collider}-$Z_1$ on $\mathcal{P}$ is in $\mathbf{A}_{XY}$; or
    \item\label{item:z1_collider_2} No \textit{collider}-$Z_1$ on $\mathcal{P}$ nor any of its descendants is in $\mathbf{A}_{XY}$.
\end{enumerate}
Note that if \ref{item:z1_collider_1} is met but \ref{item:z1_collider_2} is not (e.g., a  \textit{collider}-$Z_1$ is in $\mathbf{A}_{XY}$ but so is a non-\textit{collider}-$Z_1$), $\mathcal{P}$ is still blocked by adjusting for $\mathbf{A}_{XY}$. To prove that $\mathbf{A}_{XY}$ satisfies either \ref{item:z1_collider_1} or \ref{item:z1_collider_2}, we introduce the following propositions.

\begin{proposition}
    If a $Z_4$ shares an active path with any $Z_1$ on $\mathcal{P}$ such that $Z_4 \nind Z_1$, that $Z_4$ must form a $v$-structure $Z_4 \cdots \rightarrow Z_1 \leftarrow \cdots Z_1'$, where $Z_1'$  lies between $Z_1$ and $X$ on $\mathcal{P}$. If not, $Z_4$ would share an active path with $X$, which violates the definition of $Z_4$ (Definition \ref{def:z4}). In Figure \ref{fig:z4_z5_z1_paths} (right-hand DAG), examples include $Z_4 \rightarrow Z_1^3 \leftarrow Z_1^2$ and $Z_4 \rightarrow Z_1^3 \leftarrow Z_1^5$. Together with Definition \ref{def:z4}, this proposition implies that no $Z_4$ will ever be marginally dependent on a $Z_1$ that is directly adjacent to $X$. \label{prop:z4_z1_collider}
\end{proposition}

\begin{proposition}
    If a $Z_5$ shares an active path with any $Z_1$ on $\mathcal{P}$ such that $Z_5 \nind Z_1$, that $Z_5$ must form a $v$-structure $Z_5 \cdots \rightarrow Z_1 \leftarrow \cdots Z_1'$, where $Z_1'$  lies between $Z_1$ and $Y$ on $\mathcal{P}$. If not, $Z_5$ would share an active path with $Y$, which violates the definition of $Z_5$ (Definition \ref{def:z5}). In Figure \ref{fig:z4_z5_z1_paths} (right-hand DAG), examples include $Z_5 \rightarrow Z_1^1 \leftarrow Z_1^2$ and $Z_5 \rightarrow Z_1^1 \leftarrow Z_1^4$. Together with Definition \ref{def:z5}, this proposition implies that no $Z_5$ will ever be marginally dependent on a $Z_1$ that is directly adjacent to $Y$.\label{prop:z5_z1_collider} 
\end{proposition}

\begin{proposition} [A single $Z_1$ cannot be a collider for a $Z_4$ and a $Z_5$] \label{prop:z4_z5_z1_collider}
    %Given Propositions \ref{prop:z4_z1_collider} and \ref{prop:z5_z1_collider}, any backdoor path containing a $Z_1$ that shares an active path with either a $Z_4$ or a $Z_5$ must also contain a $Z_1$ that acts as a collider such that that the paths from $Z_4$ to $X$ and from $Z_5$ to $Y$ are inactive. 
    If a single $Z_1$ was a collider for $Z_4$ and $Z_5$, then $Z_4$ would share an active path with $X$ and $Z_5$ would share an active path with $Y$, violating the definitions of these partitions. This proposition justifies the forbidden causal path between $Z_1^5$ and $Z_1^7$ in Figure \ref{fig:z4_z5_z1_paths} (left-hand DAG).
\end{proposition}

\begin{proposition}[The \textit{root}-$Z_1$ of a backdoor path will never be marginally dependent on a $Z_4$ nor a $Z_5$] \label{prop:root_ind_z4_z5} As all \textit{root}-$Z_1$ are causal for both $X$ and $Y$, marginal dependence on either a $Z_4$ or a $Z_5$ would violate Propositions \ref{prop:z4_z1_collider}, \ref{prop:z5_z1_collider}, and \ref{prop:z4_z5_z1_collider}.
\end{proposition}

\begin{lemma}
[LDP is guaranteed to correctly label at least one $Z_1$ per backdoor path, i.e., the \textit{root}-$Z_1$] \label{lemma:catch_one_z1_per_path}
\end{lemma}
\begin{proof}
    Any $Z_1$ that is not marginally dependent on any $Z_4$ nor $Z_5$ will not be incorrectly placed in $\z_{\textsc{Post}}$ at Step 4 and will be placed in $\z_1$ at Step 6 or Step 7. Per Proposition \ref{prop:root_ind_z4_z5}, the \textit{root}-$Z_1$ of a backdoor path will never be marginally dependent on a $Z_4$ nor a $Z_5$. As all backdoor paths must have a \textit{root}-$Z_1$, then LDP is guaranteed to correctly label at least one $Z_1$ per backdoor path. 
\end{proof}

Proof of Lemma \ref{lemma:catch_one_z1_per_path} shows that LDP is guaranteed to block any backdoor path with only a single $Z_1$ that is adjacent to both $X$ and $Y$ (e.g., $Z_1^1$ in the left-hand DAG of Figure \ref{fig:z4_z5_z1_paths}). Proof of Lemma \ref{lemma:catch_one_z1_per_path} is almost proof of \ref{item:z1_collider_1} and \ref{item:z1_collider_2} for more complex backdoor paths, but with one missing link: a single $Z_1$ can act simultaneously as a \textit{root}-$Z_1$ for one backdoor path 
and as a \textit{collider}-$Z_1$ for an overlapping backdoor path. This case is exemplified by node $Z_1^2$ in Figure \ref{fig:z4_z5_z1_paths} (right-hand DAG). To fully prove \ref{item:z1_collider_1} and \ref{item:z1_collider_2}, we conclude with Lemma \ref{lemma:final}.

\begin{lemma}[Adjustment sets returned by LDP satisfy \ref{item:z1_collider_1} and \ref{item:z1_collider_2}] \label{lemma:final}
\end{lemma}

\begin{proof}
    Let $\mathcal{P}$ be a single backdoor path in $\g$. To prove Lemma \ref{lemma:final}, we will prove that if any  \textit{collider}-$Z_1$ on $\mathcal{P}$ is contained in $\mathbf{A}_{XY}$, then $\mathbf{A}_{XY}$ will also contain a non-\textit{collider}-$Z_1$ on $\mathcal{P}$. To do so, it suffices to prove that LDP correctly labels at least one \textit{root}-$Z_1$ on $\mathcal{P}$ that is not also a \textit{collider}-$Z_1$ for an overlapping backdoor path. Observe that any \textit{collider}-$Z_1$ $Z_1^*$ must be a descendant of two \textit{root}-$Z_1$ that are not \textit{collider}-$Z_1$ for any other path, however long the indirect paths to these roots are. Even if $Z_1^*$ is retained in $\mathbf{A}_{XY}$, so will its ancestors that are \textit{root}-$Z_1$ (per Lemma \ref{lemma:catch_one_z1_per_path}). Thus, even when \ref{item:z1_collider_2} goes unsatisfied, $\mathbf{A}_{XY}$ is guaranteed to satisfy \ref{item:z1_collider_1}. 
\end{proof}

Figure \ref{fig:z4_z5_z1_paths} provides an illustrative example in the right-hand DAG. There, $Z_1^2$ is a \textit{root}-$Z_1$ for backdoor path $X - Z_1^1 - Z_1^2 - Z_1^3 - Y$ but is a \textit{collider}-$Z_1$ for root $Z_1^4$ and root $Z_1^5$. Even though $Z_1^2$ is in $\mathbf{A}_{XY}$ (per Lemma \ref{lemma:catch_one_z1_per_path}), so are $Z_1^4$ and $Z_1^5$ (also per Lemma \ref{lemma:catch_one_z1_per_path}). Thus, \ref{item:z1_collider_1} and \ref{item:z1_collider_2} are satisfied by $\mathbf{A}_{XY}$.
